# Supplementary material for: Pressure Dependent Electronic Structure in CeRh$_6$Ge$_4$
Source: arXiv:2011.14256 source file (2020-11-29)
Supplement: Supplementary file 1 [file si.pdf]

# Supplementary Information: Pressure Dependent Electronic Structure in $CeRh_6Ge_4$

Chao Cao[1,2,*] and Jian-Xin Zhu[3,†]

[1]*Condensed Matter Group, Department of Physics, Hangzhou Normal University, Hangzhou 310036, P. R. China*
[2]*Center for Correlated Matter, Zhejiang University, Hangzhou 310058, China*
[3]*Theoretical Division and Center for Integrated Nanotechnologies, Los Alamos National Laboratory, Los Alamos, New Mexico 87545, USA*

(Dated: November 27, 2020)

## CALCULATION DETAILS OF DFT AND DMFT

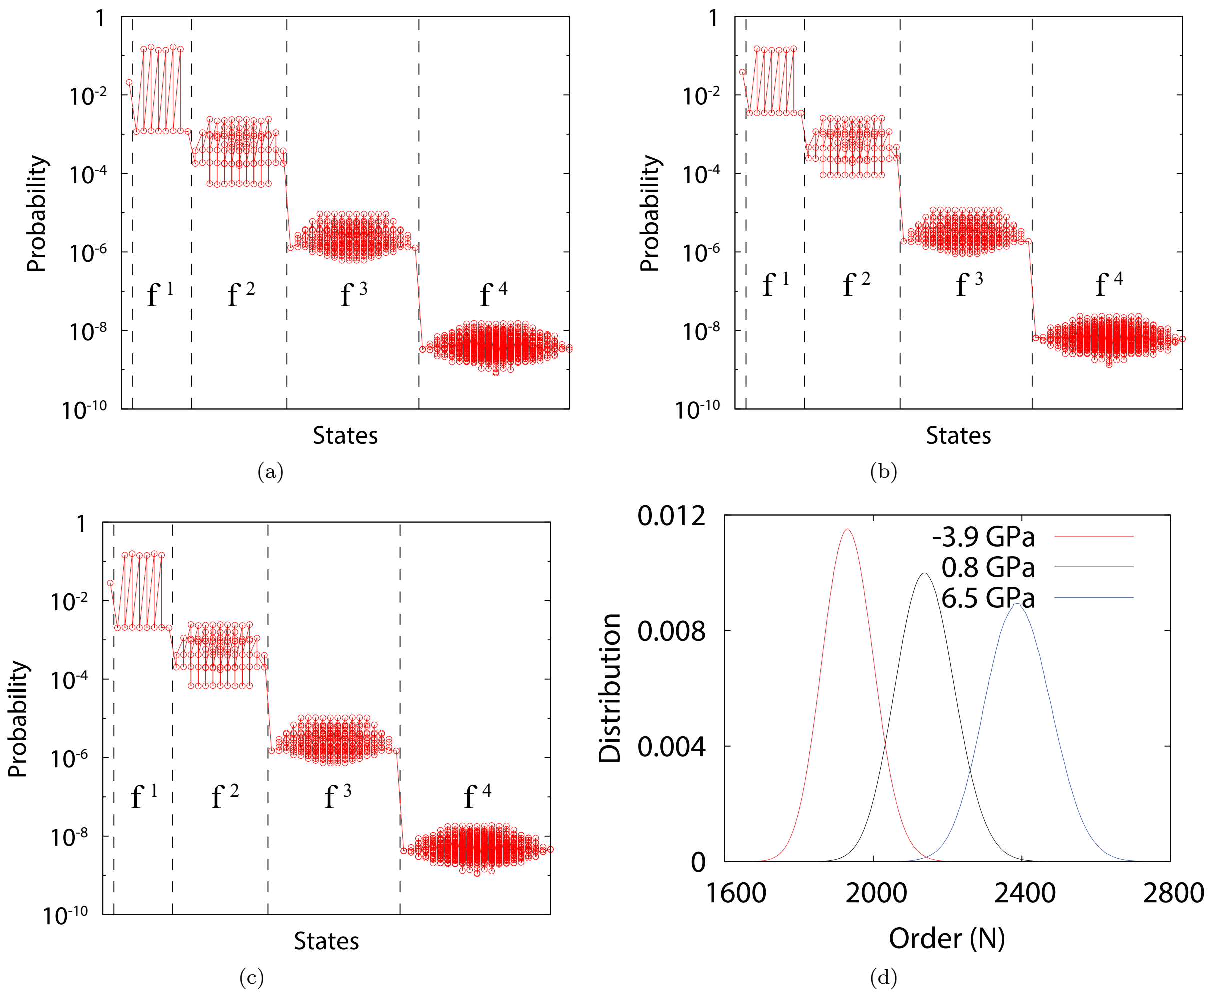


FIG. S-1: (a-c) Probabilities of many-body states at 6 K at (a) −3.9 GPa, (b) 0.8 GPa and (c) 6.5 GPa. (d) Distribution of perturbation order in these calculations.

The DFT calculations were performed using full-potential linearized augmented plane-wave (FP-LAPW) method as implemented in Wien2k code [1], and cross-checked with plane-wave projected augmented wave method using VASP [2]. The $RK_{\max}$ was set to 9, and a dense $12 \times 12 \times 19$ Γ-centered K-mesh was used for Brillouin zone integration. In VASP, the plane-wave basis energy cut-off was chosen to be 480 eV. In all calculations, the spin-orbit coupling (SOC) was included as a second variation to the total energy Hamiltonian.

The DFT+DMFT calculations were performed by using EDMFTF package [3–5]. To consider the strong correlation effects on Ce-4$f$ electrons, we have employed the local Coulomb interaction $U$=6.0 eV and $J_H$=0.7 eV (corresponding

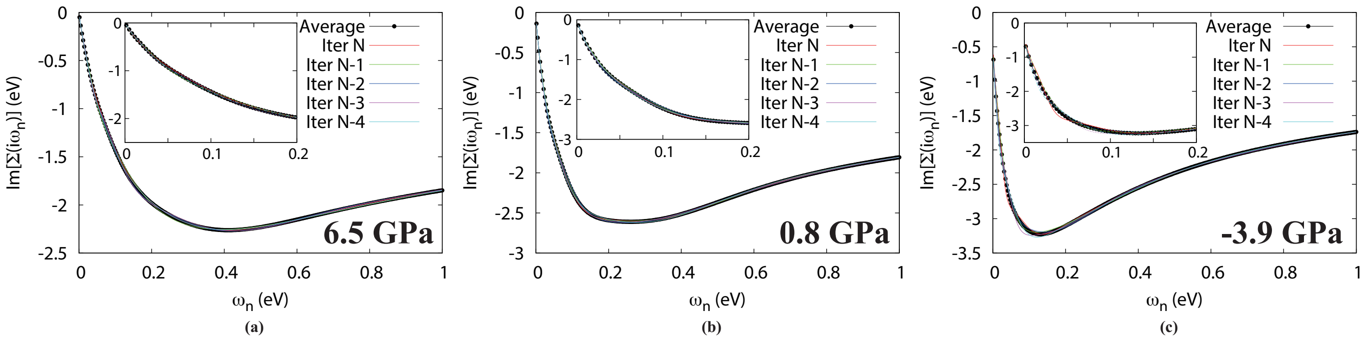


FIG. S-2: Self energies at 6 K at different pressures.

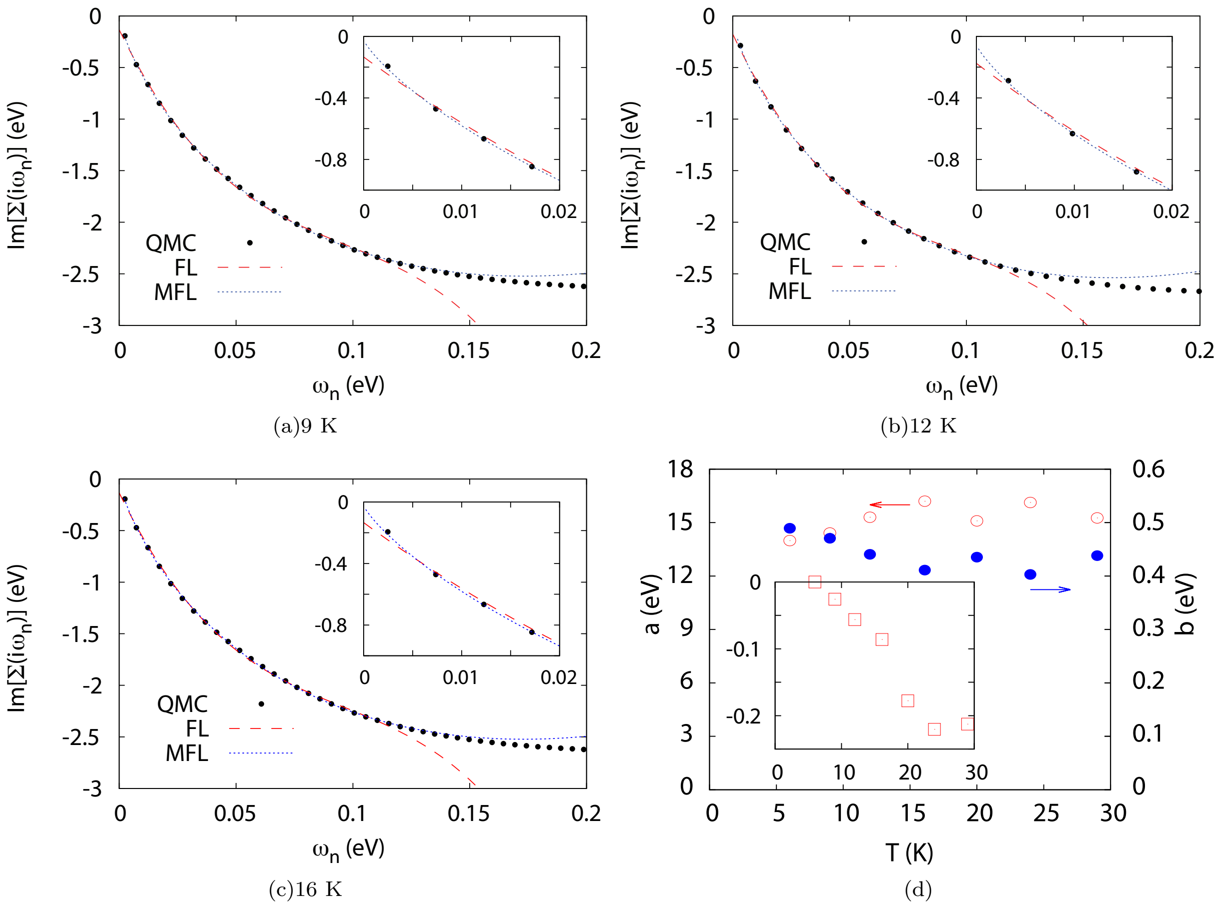


FIG. S-3: Fittings of (a) 9 K, (b) 12 K, (c) 16.1 K self-energies at 0.8 GPa. (d) Temperature dependence of fitted coefficient $a$ and $b$ in MFL form $c + a\omega_n \ln(\omega_n/b)$. The inset of panel (d) shows the temperature dependence of $c$, which is set to be 0 at 6 K.

to $F^0$=6.0 eV, $F^2$=8.345 eV, $F^4$=5.5747 eV, $F^6$=4.1226 eV). The low-energy Hamiltonian was obtained by projecting the states within [-10.0, 10.0] eV with respect to the Fermi level, which contains more than 140 states. The crystal field splitting (CEF) was considered at the DMFT (lattice) level, and 6 degenerate $J = 5/2$ orbitals and 8 degenerate $J = 7/2$ orbitals are considered in the quantum impurity solver. The continuous-time hybridization-expansion quantum Monte Carlo (CTQMC) impurity solver was employed, and the full Coulomb interaction matrix was used. A singular value decomposition basis expansion to the Green's function up to $l$=29 was used in our calculations, and nominal double counting with $n_f^0 = 1$ was chosen. In Fig. S-1, we show the probabilities of many-body states at 6 K at $-3.9$ GPa, 0.8 GPa, and 6.5 GPa. The probability of $n_f = 4$ states is 2 orders of magnitude smaller than that of $n_f = 3$ states, and constitutes less than 0.001% of the total probability. We thus restricted the impurity electron occupation

within [0, 3]. The local magnetic susceptibility is calculated by the impurity solver using $\chi_{\rm loc} = \chi^{zz}_{\rm imp}(\Omega = 0) = \int_0^\beta d\tau \, \langle J^z(\tau) J^z(0) \rangle$.

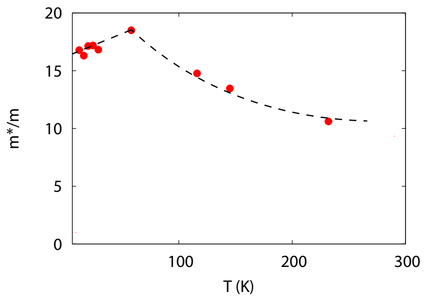

(a)13.1 GPa

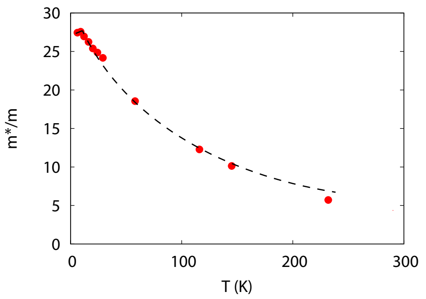

(b)6.5 GPa

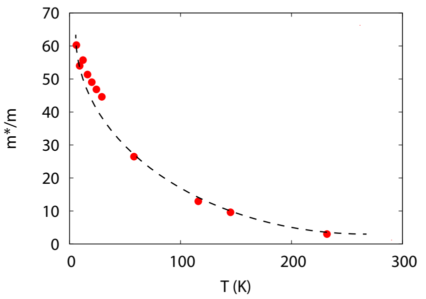

(c)0.8 GPa

FIG. S-4: Temperature dependent effective mass $m*/m$ at different pressures. The dashed lines are guidance to the eyes.

For calculations below 20 K, we used 192 CPU-core and $1{\times}10^9 \sim 1 \times 10^{10}$ QMC steps for each QMC run. The calculations converge after 30∼60 DMFT iterations, each consists of 1 QMC run and maximally 20 charge iterations. For calculations at higher temperatures, we used 96 CPU-core and $2 \times 10^8 \sim 2 \times 10^9$ QMC steps for each QMC run. These calculations converge after 20∼40 DMFT iterations, each also contain 1 QMC run and maximally 20 charge iterations. In each case, another 5 DMFT iterations were employed to calculate the averaged self-energy and the statistics for impurity occupation $n_f$ as well as the magnetic susceptibility $\chi_{\rm loc}$. We show also the distribution of perturbation order at 6 K at different pressure in Fig. S-1(d). The perturbation beyond 2800 is already quite small. Therefore, the maximum perturbation order is truncated beyond 4800 at 6 K.

## SELF-ENERGIES AND EFFECTIVE MASS

We show the last 5 iterations of lowest temperature DMFT self energy and their averages in Fig. S-2. For 0.8 GPa and 6.5 GPa results, the self-energies from the last 5 iterations are very well converged. For the −3.9 GPa calculation, the self energies experience larger fluctuations, but are still converged, and the local-moment behavior ($\mathrm{Im}[\Sigma(\omega=0)] < 0$) is apparent and consistent. In addition, we show also 3 additional fittings to the low-frequency behaviors of self-energies at 0.8 GPa in Fig. S-3. In these fittings, the marginal Fermi-liquid form is supplemented with an additional constant for the thermal effect, i.e. $\mathrm{Im}[\Sigma(i\omega_n)] \approx c + a\omega_n \ln(\omega_n/b)$, and the fitting range in both MFL and FL cases are between $\omega \in [0, 0.12]$ eV. In each case, the MFL fitting is better than the FL fitting, especially for $\omega \in [0, 0.02]$ eV and [0.1, 0.15] eV. In Fig. S-3(d), we show the temperature dependence of the fitted parameters in the MFL case. The fitted $a$ ($b$) are around 15.2 eV (0.44 eV), respectively; while $c$ systematically reduces as the temperature reduces. This robustness of the improvement of MFL over FL against the lowering temperature suggests the predicted MFL is expected to hold for temperatures below 6 K as well.

The effective mass $m^*/m = 1/Z$ and zero-frequency self-energy $\mathrm{Im}[\Sigma(\omega=0)]$ in the text are obtained by fitting $\mathrm{Im}[\Sigma(i\omega_n)]$ up to the first 6 Matsubara frequencies ($\omega_1$ to $\omega_6$) to a cubic polynomial function $\mathrm{Im}[\Sigma(\omega=0)] + (Z^{-1} - 1)\omega + c\omega^2 + d\omega^3$. We show the calculated effective mass in Fig. S-4. For −3.9 GPa and −8.3 GPa, although such fitting is still possible at low temperatures, the conduction electron states dominate the electron states near the Fermi level $E_F$ (refer to next section), and therefore the Ce-4$f$ effective mass is not relevant.

## ELECTRONIC DENSITY OF STATES AND FERMI SURFACES

We show the DOS of $\mathrm{CeRh_6Ge_4}$ at −3.9 GPa to 13.1 GPa in Fig. S-5. At high temperature (232K) [Fig. S-5(a)], Ce-4$f$ states are localized except at 13.1 GPa. Therefore, they have negligible contribution to the electronic states at the Fermi level. On the other hand, at 13.1 GPa, a quasiparticle coherence peak already starts to form at such a high temperature. At low temperature (12 K) [Fig. S-5(b)], Ce-4$f$ states remain localized at −3.9 GPa. At other pressure values, the coherence peaks are sharp and Ce-4$f$ states are itinerant and dominate the contribution to the DOS near the Fermi level. Therefore, at pressures higher than 0.8 GPa, it is expected that the effective mass should mostly contributed by the Ce-4$f$ states; while at lower pressures, the normal conduction electrons dominate.

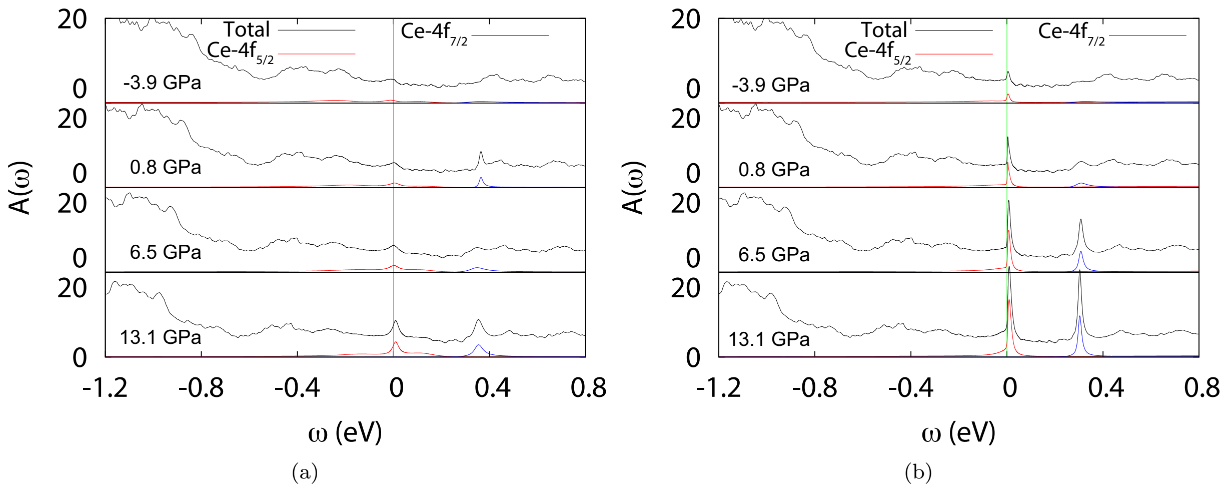


FIG. S-5: Electronic density of states of $CeRh_6Ge_4$ at different pressures at (a) 232K and (b) 12K.

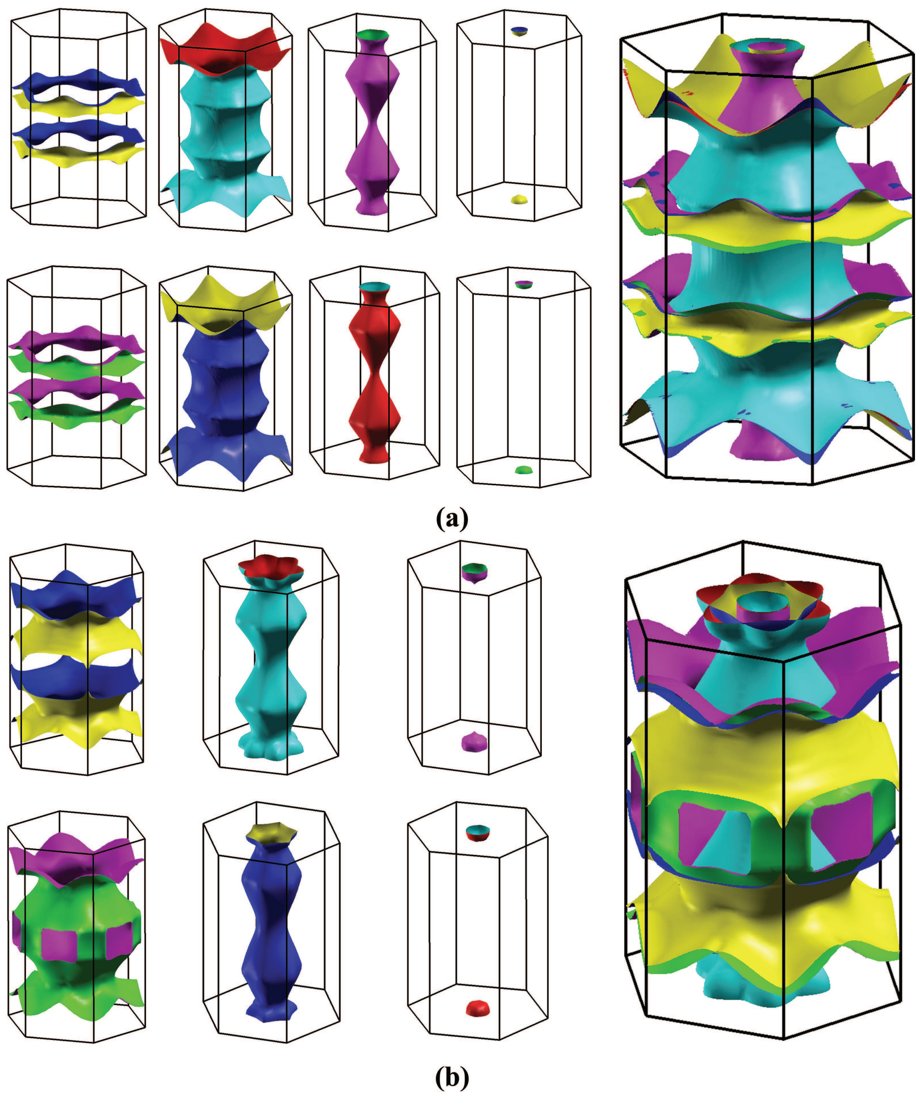


FIG. S-6: Fermi surfaces at (a) -3.9 GPa and (b) 6.5 GPa, calculated at 6K.

We show in Fig. S-6 the Fermi surface topology of $CeRh_6Ge_4$ at $-3.9$ GPa and 6.5 GPa calculated at 6 K.At $-3.9$ GPa, the Ce-4$f$ electrons are localized, and the Fermi surface consists of 8 sheets [Fig. S-6(a)], among which there exist two tiny pockets around A; at 6.5 GPa, when the Ce-4$f$ electrons are in the itinerant state [Fig. S-6(b)], the Fermi surface consists of 6 sheets. Moreover, in the localized states, the 8 sheets contribute 0.045 $h$, 0.058 $h$, 0.487 $h$, 0.508 $h$, 0.065 $e$ 0.055 $e$, 0.001 $e$, and 0.001 $e$, respectively; while in the itinerant states, the 6 sheets contribute 0.184 $h$, 0.282 $h$, 0.162 $e$, 0.119 $e$, 0.004 $e$ and 0.003 $e$, respectively. As a result, from local to itinerant Ce-4$f$ electrons, the Fermi surfaces are enlarged as expected.

* E-mail address: ccao@hznu.edu.cn
† E-mail address: jxzhu@lanl.gov

[1] K. Schwarz, P. Blaha, and G. K. H. Madsen, Computer Physics Communications **147**, 71 (2002).
[2] G. Kresse and D. Joubert, Phys. Rev. B **59**, 1758 (1999).
[3] K. Haule, C.-H. Yee, and K. Kim, Phys. Rev. B **81**, 195107 (2010).
[4] A. Georges, G. Kotliar, W. Krauth, and M. J. Rozenberg, Rev. Mod. Phys. **68**, 13 (1996).
[5] G. Kotliar, S. Y. Savrasov, K. Haule, V. S. Oudovenko, O. Parcollet, and C. A. Marianetti, Rev. Mod. Phys. **78**, 865 (2006).
